# Supplementary material for: XCRYPT: Accelerating Lattice Based Cryptography with Memristor Crossbar Arrays
Source: arXiv:2302.00095 source file (2023-01-31)
Supplement: Supplementary file 1 [file appendix.tex]

\appendix

\section{Appendix}
\label{append}

\subsection{Notations}
\label{subsec:notations}

We use $\Z_q$ to denote the ring of integers modulo integer $q$, i.e., integers in $[0,q)$. $\Z_q[x]$ denotes the ring of polynomials in $x$ with coefficients in $[0,q)$. $R_q = \Z_q[x] / (x^n + 1)$ is the more constrained ring of polynomials of degree $n$, where $n$ is a fixed power of 2 (we use $n=256$).  During computations, if a polynomial's degree exceeds $n$, it is divided by $x^n+1$ to lower its degree (essentially, like a modulo operation for polynomials).  Formally stated, this set of polynomials is referred to as the quotient ring $R_q = \Z_q[x]/(x^n+1)$. For instance, consider a polynomial $\Z_q[x] = (3+2x^2+x^4+10x^5+6x^6)$, and $n=4$; $R_q$ is remainders of Euclidean divisions of $\Z_q[x]$ by $(x^4+1)$, which is $(3+2x^2-(1+10x^1+6x^2)) = 2-10x^1-4x^2$.

For ring $R_q$, $R_q^{l \times k}$ denotes the ring of $l \times k$-matrices over $R_q$, i.e., each element of the matrix is a polynomial. 
%Mod operator is applied over coefficients of $R$. 
Polynomials are written without markup, %vectors are bold lower case, and 
and matrices are denoted with bold upper case. 
$\beta_{\mu}$ denotes a centered binomial distribution with parameter $\mu$, resulting in samples in the interval $[-\mu/2,\mu/2]$.

\subsection{Formal Expressions for LBC Algorithms}
\label{subsec:formal}

\noindent {\bf Standard LWE:}
Randomly chosen $\vec{s} \in \Z_{q}^n$ ($\Z_q^n$ denotes a vector of dimension $n$ with its values in $\Z_q$).
Multiply $\vec{s}$ with $m$ random vectors ($\vec{a}_i \in \Z_q^n$), and add a small error $e_i$, to generate $\vec{b}$.  This is formally represented as:
$\left( \vec{a}_i, b_i = \langle \vec{a},\vec{s} \rangle + e_i \right) \in \Z_q^n \times \Z_q; \quad (\mat{A}, \vec{b}) = (\vec{a}_i, b_i)_{i=1}^m$

\noindent {\bf Ring LWE:}
Samples are drawn as polynomials in the ring $R_q = \Z_q[x]/(x^n+1)$.

\noindent {\bf Module LWR:}
$\left( \vec{a}, b= \lfloor \frac{p}{q} \langle \vec{a},\vec{s} \rangle \rceil_p \right) \in \R_q^{l \times 1} \times \R_p$

\noindent {\bf SABER Parameters:}
SABER defines its PKE parameter set as follows: security parameter $n=256$, module rank $l=3$, modulus $q=2^{13}$, rounding factors $p=2^{10}$ and $T=2^{4}$, $\mu=8$. SABER also uses three constants: 1) polynomial $h_1 \in R_q$ with coefficients as $2^{\log{q}-\log{p}-1}$, 2) a vector $\vec{h} \in R_q^{l \times 1}$ where each polynomial is $h_1$, and 3) polynomial $h_2 \in R_q$ with coefficients as $(2^{\log{p}-2}-2^{\log{p}-\log{T}-1}+2^{\log{q}-\log{p}-1})$. These constants are added in order to replace rounding with simple bit shifts.
